# Supplementary material for: An interlayer with low solubility for lithium enhances tolerance to dendrite growth in solid state electrolytes
Source: arXiv:2001.06276 ancillary file (2020-01-17)
Supplement: Supplementary file 1 [file Raj_SI_17Jan2020_C.pdf]

# Supplementary Information

# An interlayer with low solubility for lithium enhances tolerance to dendrite growth in solid state electrolytes

Vikalp Raj, Varun R Kankanallu, Bibhatsu Kuiri, Naga Phani B. Aetukuri*

Solid State and Structural Chemistry Unit, Indian Institute of Science,
Bangalore, 560012, Karnataka, India

*Corresponding Author; E-mail: phani@iisc.ac.in

## Contents

**1 Experimental Methods** **2**

1.1 Synthesis of Ta doped LLZO . . . . . . . . . . . . . . . . . . . . . . . . . . . . 2

1.2 Interlayer Deposition . . . . . . . . . . . . . . . . . . . . . . . . . . . . . . 3

1.3 Cell fabrication, assembly and measurements . . . . . . . . . . . . . . . . . . . . 3

1.4 Critical Current Density Experiments . . . . . . . . . . . . . . . . . . . . . . . 5

1.5 Ionic conductivity of LLZTO pellets . . . . . . . . . . . . . . . . . . . . . . . . 6

1.6 Interfacial Impedance Calculations . . . . . . . . . . . . . . . . . . . . . . . . 9

1.7 Sample Preparation for Cross-Sectional SEM . . . . . . . . . . . . . . . . . . . 9

1.8 Measuring lithium nucleation overpotentials on Al and W . . . . . . . . . . . . 11

1.9 Current Density Simulations . . . . . . . . . . . . . . . . . . . . . . . . . . . 11

**2 Supplementary Figures and Tables** **13**

# 1 Experimental Methods

## 1.1 Synthesis of Ta doped LLZO

Tantalum doped LLZO with the nominal chemical formula $Li_{7-x}La_3Zr_{2-x}Ta_xO_{12}(LLZTO)$ is the preferred solid state electrolyte for all the experiments presented in this work. Tantalum was chosen as the dopant because it was shown to be stable to potentials of up to 6 V v/s $Li^+$/Li. Also, it has been shown that tantalum substitution on zirconium sites will not hinder Li-ion mobility leading to ionic conductivities of 5E-4 S/cm and higher (*1, 2*). We employed a solid state synthesis technique, based on a previously reported synthetic procedure by Prof. Goodenough's research group (*3*). In this procedure, first, stoichiometric amounts of $La_2O_3$ (99.9 % merck), $ZrO_2$ (99 % trace metal basis, merck), $Ta_2O_5$ (99 % trace metal basis, sigma aldrich) and 50% excess $Li_2CO_3$ (99 % ACS reagent,merck) were thoroughly mixed using an agate mortar and pestle. Charge calculations for synthesis are based on a targeted tantalum doping level of x=0.6. An excess of lithium carbonate was taken to counter Li loss during sintering and also to aid the formation of Li-Al melt which will assist in the densification of pellets (*4*). The source of aluminum for densification is through its diffusive mixing from the alumina crucible used for sintering the chemical mixture. The mixture, in an alumina boat, was annealed at 900 °C for 12 hours in a muffle furnace. The furnace was heated and cooled at a rate of 200 °C per hour. After cooling, the powder was again mixed using a mortar and pestle. The homogenized mixture is then pressed into pellets that are ~1.5 mm in thickness and 13 mm in diameter, using a cold hydraulic press. The green pellets were placed in an alumina crucible while being pre-layered and covered with a sacrificial powder with the same composition as the one used for making pellets. The pellet-powder assembly is then sintered at a temperature of 1140°C for 16 hours. Sintered pellets were then dry polished sequentially with 200, 400, 600, 800, 1000, 1200 and 2000 grit SiC sandpaper. The dry polished pellets were then wet polished with 0.1 $\mu$m diamond

suspension (diamond powder suspended in olive oil). All polishing steps were done in ambient laboratory environment. Finally, all polished pellets were washed with tetrahydrofuran (THF) and stored in argon filled glove box until being used for cell assembly or interlayer deposition. The average pellet density, calculated using the Archimedes' principle with ethanol as a the solvent, was found to be 88-90 % of the theoretical density.

## 1.2 Interlayer Deposition

For interlayer deposition, polished pellets were transferred to a sealable pellet carrier inside an argon filled glove box operating at <0.5 ppm $H_2O$ and <0.1 ppm $O_2$. The pellets from the carrier were transferred to an Anelva sputter deposition system while ensuring that the pellets are exposed to ambient atmosphere for less than a few minutes. All interlayers viz., 50 nm Al, 30 nm W, and 30 nm Mo were deposited using DC magnetron sputtering in the Anelva sputtering tool on both sides of the pellet. After deposition, the substrates were transferred to the pellet carrier while minimizing the time where they are exposed to ambient. The pellet carrier is finally transferred to the glove box with pellets having interlayers. Similar approach is used for preparing cells for testing ion conductivity of the solid state electrolyte using Au blocking electrodes. 100 nm Au blocking electrodes were deposited on both sides of the pellet using DC magnetron sputtering. Patterned interlayer cells, where a small area on the pellet does not have the interlayer, are prepared by depositing an interlayer material on one side as stated above. For the other side, a tiny drop-casted region of polymethyl methacrylate (PMMA) was used to mask off the region before aluminum deposition. The PMMA used for masking is then dissolved in acetone to leave behind a region without the interlayer.

## 1.3 Cell fabrication, assembly and measurements

Symmetric Li-Li half cells with and without interlayers: Li/LLZTO/Li, Li/Al/LLZTO/Al/Li, Li/W/LLZTO/W/Li and Li/Mo/LLZTO/Mo/Li cells were assembled in an argon filled glove box operating at <0.5 ppm $H_2O$ and <0.1 ppm $O_2$. The cells were assembled from pellets

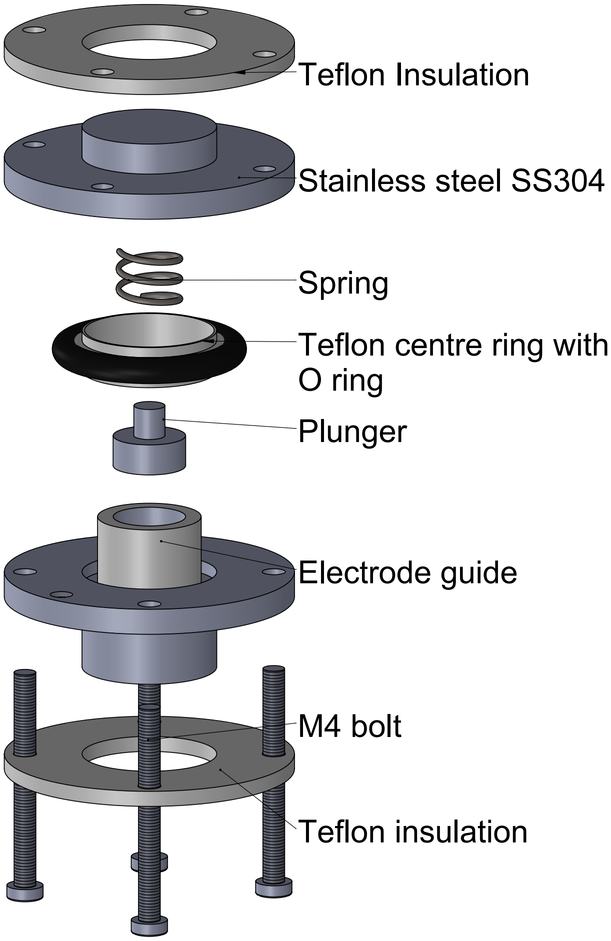


**Figure S1 | Custom-built electrochemical cell.** A CAD rendering of a custom-built cell used for performing electrochemical measurements reported in this work. The different components of the cell are labeled in the drawing.

prepared using the procedure detailed in section 1.1 and 1.2. A fresh rolled lithium foil with $\sim$8 mm diameter and $\sim$ 100 microns in thickness was stuck on each side of the pellets with or without an Al or W or Mo interlayer. A stainless disc that is 8 mm in diameter and 1 mm in thickness is then placed on top of the lithium on each side of the pellet. This entire assembly was then placed on a hot plate at 300 °C and heated for 12 hours. Based on measurements using a thermocouple, the half cell components are estimated to reach a temperature of 230-250 °C

during this cell formation step. After 12 hours, the formed cells are taken off the hot plate and allowed to cool to room temperature. After cooling down, the Li-Li half cell is placed into a custom-built cell holder (Fig. S1) and sealed inside the glove box. The entire cell assembly is taken out of the glove box for electrochemical testing. Electrochemical testing was then performed using a PARSTAT MC2000A or MC200 potentiostat in a two-electrode geometry. The potentiostatic electrochemical impedance measurements presented in this manuscript were all performed over a frequency range of 100 mHz to 100 kHz using an excitation voltage of 20 mV.

For experiments performed using Li-ion blocking Au/LLZTO/Au half-cells, the cells were assembled without any lithium on the Au layers. Since there is no lithium, the cells are not heated to 300 °C. The rest of the procedure is identical to the assembly of symmetric Li-Li cells. (also see SI section 1.6)

## 1.4 Critical Current Density Experiments

Symmetric Li-Li cells with and without interlayers were first subjected to a galvanostatic training step. In this step, a constant current density of 100 μA/cm$^2$ is applied cyclically (alternate lithium plating and stripping cycles) for 24 hours with 5 minutes each for a plate and strip cycle. The data from this training step is also used to calculate interfacial impedance for each cell. For interfacial impedance calculations, ion conductivity is assumed to be nearly identical for all pellets and was calculated based on impedance measurements performed on Li-ion blocking Au/LLZO/Au cells.

After the galvanostatic training step, unless otherwise mentioned, the cell is cycled at increasing current densities from 100 μA/cm$^2$ in steps of 10 μA/cm$^2$ to current densities beyond the critical current density for experiments performed at 25 °C and in steps of 20 μA/cm$^2$ for experiments performed at higher temperatures. At each current density a cell is cycled between a 5-minute plate and 5-minute strip step for 5 times. The first instance of a partial but sudden drop in potential is considered as a short and the current density when such a drop in potential

occurs is taken as the critical current density. Cross-verification using impedance measurements was done in a few cells to ascertain that this sudden drop in potential indeed corresponds to an electrical short in the cell. Cells after such soft shorts usually showed dark spots on the surfaces of the pellets possibly indicative of regions of dendrite growth. See Table. S2 for details of all samples measured for the purposes of this work.

## 1.5 Ionic conductivity of LLZTO pellets

Ionic conductivity of LLZTO pellets was measured by a standard two probe electrochemical impedance spectroscopy (EIS) measurement using gold blocking electrodes. The measurements were done over a frequency range of 1 Hz to 100 kHz with an excitation voltage of 20 mV. Temperature-dependent impedance measurements were performed to calculate activation energy for ionic conduction in LLZTO (Fig. S6) All experimental EIS data was fitted using ZSimpWin software using an equivalent circuit model shown in (Fig. S2). The ionic conductor is approximated by an ionic resistance ($R_{ion}$) in parallel with a constant phase element Q1 (*5*). A series resistor $R_s$ is used to approximate the contact and lead resistance and a series constant phase element Q2 is used to approximate the blocking nature of the gold electrodes (*6*). The average ionic conductivity of LLZTO pellets was found to be 0.5 mS/cm and the activation energy for ionic conductivity was found to be $\sim$0.36 eV.

The ionic conductivity measured by EIS was cross verified using a DC resistance measurement technique as outlined below. A list of pellet thicknesses used and stripping/plating potentials obtained from galvanostatic experiments performed at 100 $\mu$A/cm$^2$ at room temperature is given in Table S1 and plotted in Fig. S3. In such a plot, the slope of the potential versus thickness will be proportional to the ionic resistivity of the LLZTO pellet. The intercept gives an average interfacial resistance. Based on a slope of $\sim$189 mV/cm from Fig. S3 and the galvanostatic current density of 100 $\mu$A/cm$^2$, the average ionic conductivity of the pellets was calculated to be $\sim$ 0.5 mS/cm, which is in very good agreement with the calculation of ionic

conductivity based on EIS measurements. Note that ionic conductivity is given by:

$$\sigma = \frac{j}{slope} \tag{1}$$

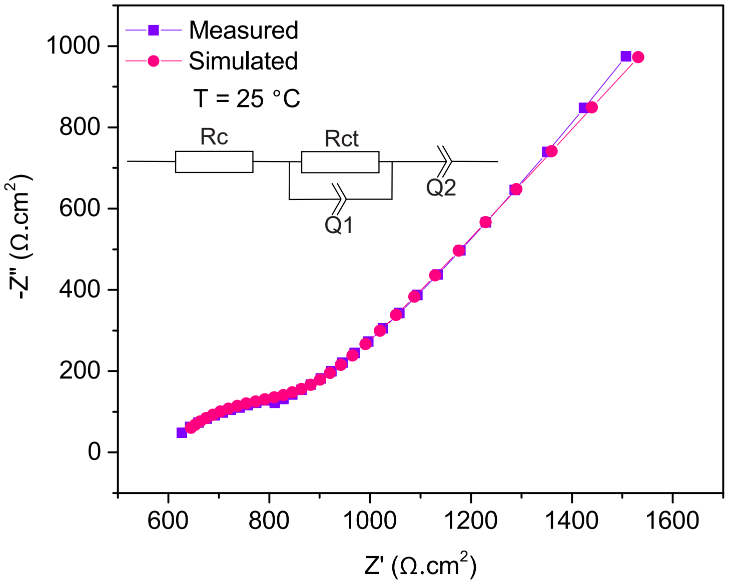


**Figure S2 | Ionic conductivity of LLZTO.** A typical Nyquist plot showing the experimental (filled squares) and fitted (filled circles) impedance data for a 1.1 mm LLZTO pellet at room temperature. The data was collected over a frequency range of 1 Hz to 100 kHz with an AC excitation voltage of 20 mV. Equivalent circuit diagram used for fitting experimental data is shown in the inset.

| Cell No. | Thickness (cm) | Over potential (mV) |
|---|---|---|
| 1 | 0.119 | 45 |
| 2 | 0.172 | 60 |
| 3 | 0.261 | 69 |
| 4 | 0.350 | 88 |
| 5 | 0.287 | 85 |
| 6 | 0.171 | 65 |
| 7 | 0.113 | 40 |
| 8 | 0.078 | 50 |
| 9 | 0.145 | 42 |
| 10 | 0.140 | 44 |
| 11 | 0.143 | 44 |

**Table. S1 | List of pellet thicknesses and associated plating/stripping potentials.** List of pellet thicknesses used and stripping/plating potentials obtained from galvanostatic experiments performed at 100 $\mu$A/cm$^2$ at room temperature.

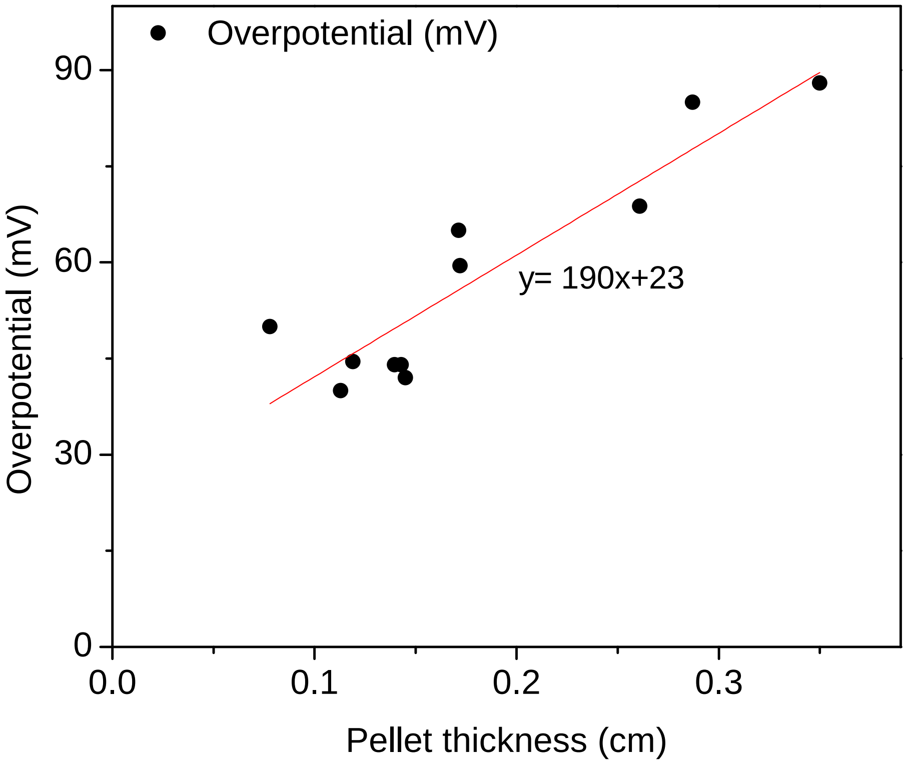


**Fig. S3 | Plating/stripping potential versus pellet thickness.** A plot of a pellet thickness versus potential obtained from galvanostatic plating/stripping experiments performed at 100 $\mu$A/cm$^2$ at room temperature.

## 1.6 Interfacial Impedance Calculations

Before a critical current density experiment, all cells were galvanostatically cycled at a current density of 100 $\mu$A/cm$^2$ for a period of 24 hours at 25 °C. Each plating and stripping cycle was performed for 5 minutes. The plating or stripping potential comprises of the potential drop due to the bulk ionic resistance and also due to the interfacial resistance. For unit area of the pellets, this statement is equivalent to:

$$\text{ASR}_{interface} = \frac{(\text{ASR}_{total} - \text{ASR}_{bulk})}{2} \tag{2}$$

$$\text{ASR}_{bulk} = \frac{l}{\sigma} \tag{3}$$

$$\text{ASR}_{total} = \frac{E}{j} \tag{4}$$

where $\text{ASR}_{interface}$, $\text{ASR}_{bulk}$, $\text{ASR}_{total}$ represent the area specific resistances due to the interface, the bulk and the total resistive contribution respectively. $l$ is the thickness of the pellet, $\sigma$ is the bulk ionic conductivity of the pellet, $E$ is the total potential drop during plating or stripping and $j$ is the current density used for galvanostatic cycling experiments. The denominator 2 in equation 2 is because interfacial resistance is assumed to be identical for both the Li/Al/LLZTO interfaces. As an example, the $\text{ASR}_{interface}$ for data shown in Fig. S4 is calculated to be $\sim$91 $\Omega$-cm$^2$. For these calculations, the average potential drop $E$ is taken to be 41 mV and $\sigma$ is taken to be 0.5 mS/cm. The thickness of the pellet, $l$, is 1.1 $mm$ and $j$ is 100 $\mu$A/cm$^2$.

## 1.7 Sample Preparation for Cross-Sectional SEM

Cross-sectional SEM was performed on cells with and without interlayers. Samples for SEM experiments were prepared by disassembling cells, in an argon-filled inert glove box with <0.5 ppm $H_2O$ and <0.1 ppm $O_2$, after electrochemical measurements. The procedure for sample preparation includes: 1) Heating cells with LLZTO pellets to 250 °C so that stainless steel current collectors can be gently removed without breaking the pellets; 2) Allowing the elec-

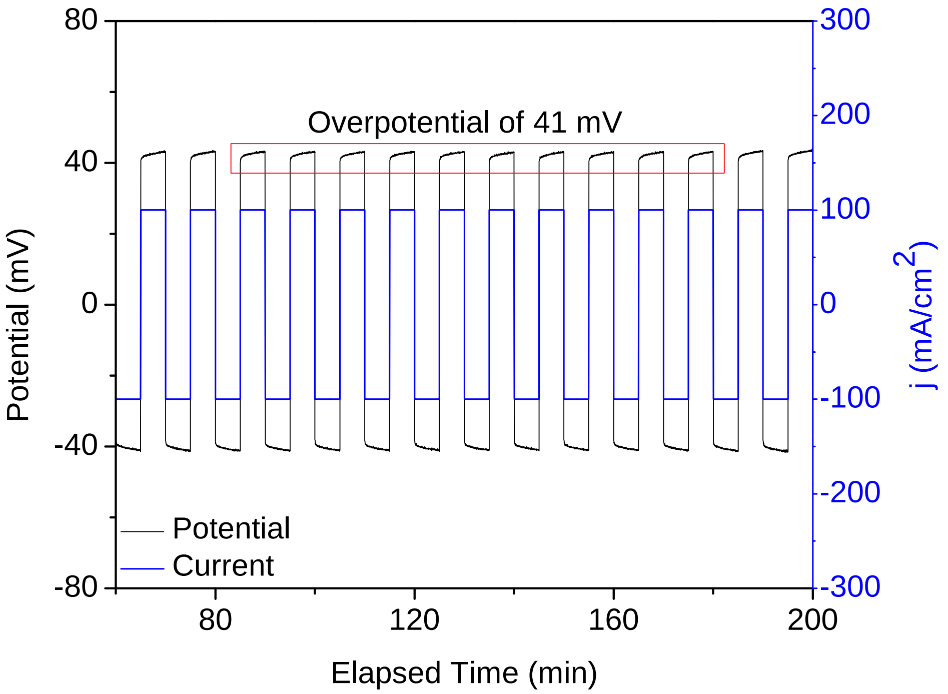


**Fig. S4 | Galvanostatic cycling of a Li/Al/LLZTO/Al/Li symmetric cell.** A plot of potential and current density versus time obtained from a galvanostatic cycling experiment performed on a Li/Al/LLZTO/Al/Li symmetric cell at a current density of 100 $\mu$A/cm$^2$ at room temperature. The plating/stripping potential for this cell is 41 mV.

trode/LLZTO/electrode assembly to cool down before the assembly is rapidly diced or snipped to expose a cross-sectional surface for SEM experiments. The samples are then mounted on an aluminum stub and transferred to a desiccator used for transporting the samples to the SEM facility. The time of exposure of samples to the ambient atmosphere during the transfer from a desiccator to the SEM sample transfer chamber was kept to less than a few minutes. All SEM imaging was performed on Ultra55 FE-SEM Karl Zeiss system with a beam energy of 5 kV or less. All the images presented in this work are collected using a high efficiency secondary electron SE2 detector.

## 1.8 Measuring lithium nucleation overpotentials on Al and W

A conventional liquid electrolyte cell employing 1 M lithium bis(trifluoromethanesulfonyl)imide (Li-TFSI) in 1,2 dimethoxyethane (DME) as the electrolyte was used for measuring overpotentials for lithium nucleation on aluminum and tungsten. The measurements were performed in a 2-electrode geometry with a lithium counter electrode (also functioning as a pseudo-reference electrode) and either a tungsten foil or a 200 nm aluminum on stainless steel as the working electrode. All lithium plating experiments were performed under galvanostatic conditions at a current density of 100 $\mu$A/cm$^2$. After every lithium plating step, the deposited lithium is completely stripped under galvanostatic conditions at a current density of 100 $\mu$A/cm$^2$ by allowing the lithium to strip for the same time as the lithium plating step or until the cell polarization reached a potential of 1.5 V vs $Li^+$/Li. .

## 1.9 Current Density Simulations

Finite element simulations were performed using the Electrical Current (EC) module in COMSOL. The simulations were performed in a 2D geometry for a cell with 3 $\mu$m thick lithium electrodes sandwiching a 10 $\mu$m thick slab of the ion conductor. Since the simulations are performed using the EC module, the ion-conductor is approximated by an electrical conductor with an electrical conductivity of 0.5 mS/cm. The x-axis is chosen to be along the direction of the interface between the lithium electrode and the ion conductor. The y-axis is chosen to be along the normal to the interface between the lithium electrode and the ion conductor. The external surface of one of the lithium electrodes is connected to a current source and the external surface of the other lithium electrode is connected to a current sink. The boundaries along the y-axis are assumed to be perfect insulators (see Fig. S5). A triangular void, 10 $\mu$m in length and 1 $\mu$m in height, is used for approximating a spherical void.

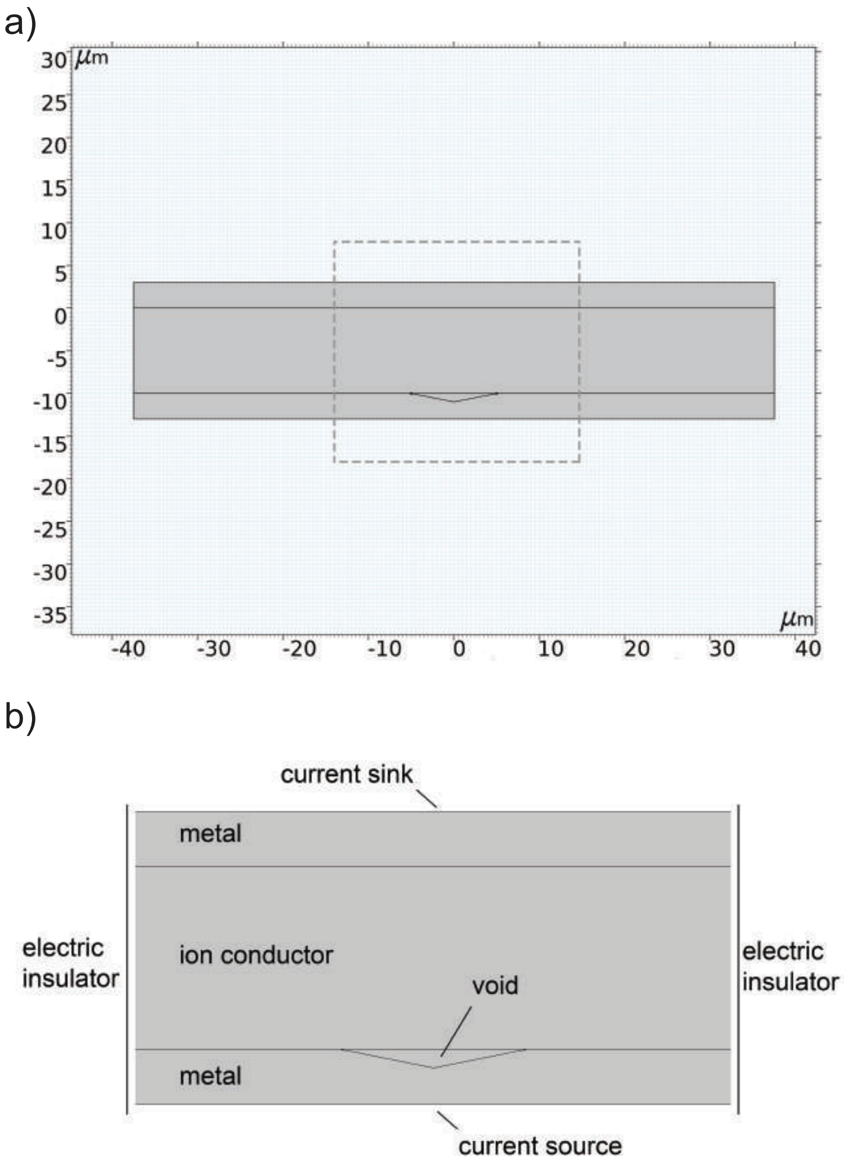


**Fig. S5 | Sample geometry used for COMSOL Simulations. a** Geometry used for modeling critical current density in the vicinity of a void. **b** is a magnified version of the same figure as in **a**. In the simulation, the external surface of the bottom lithium electrode is connected to a current source and the external surface of the top lithium electrode is connected to a current sink (ground). The other surfaces are set as electrically insulating boundaries. A triangular void, 10 $\mu$m in length and 1 $\mu$m in height is used to simulate voids at interfaces in Li/LLZTO/Li interfaces.

# 2 Supplementary Figures and Tables

## Figure S6

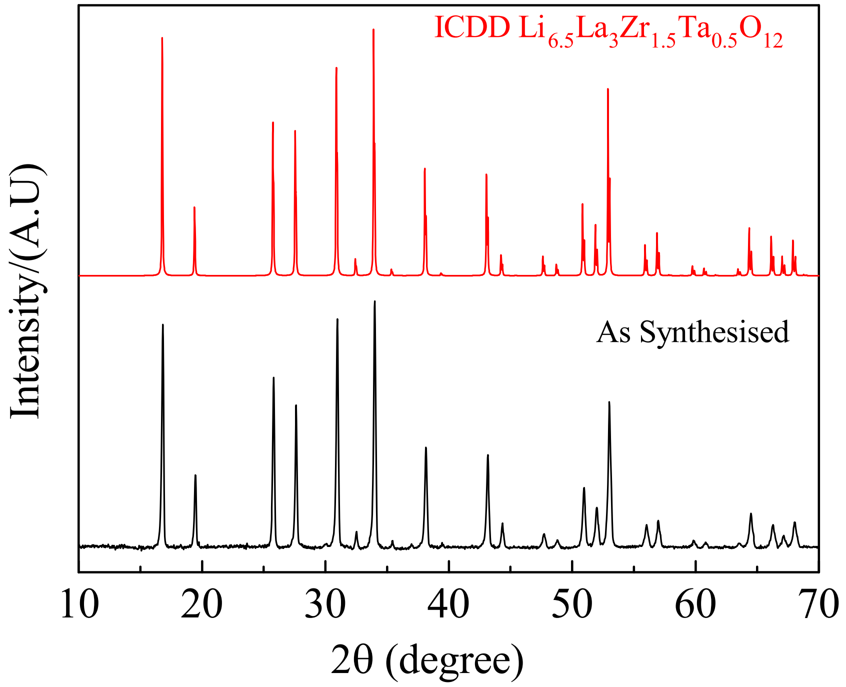


**Fig. S6 | X-ray Diffractogram of as-synthesized LLZTO. a**. A comparison of $\theta$-$2\theta$ x-ray diffractograms of as-synthesized LLZTO powder with a standard pattern of $Li_{6.5}La_3Zr_{1.5}Ta_{0.5}O_{12}$. Clearly, there is a good match with the standard diffractogram which is indicative of the structural quality of LLZTO used in these experiments.

## Figure S7

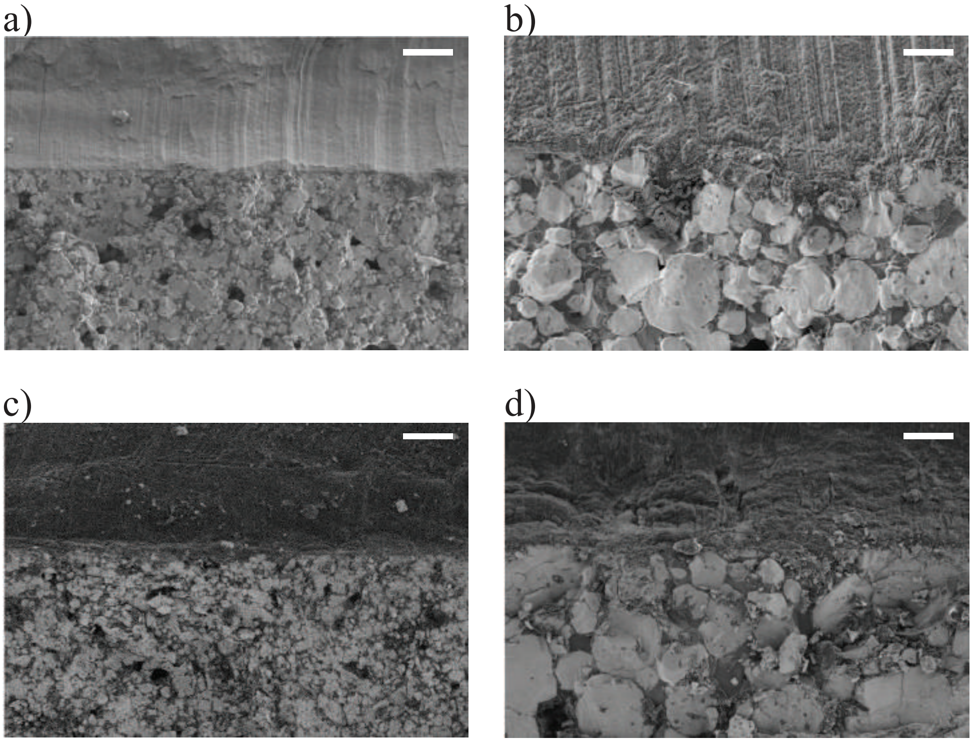


**Fig. S7 | Interface quality in cells with interlayers.** Cross-sectional SEM images of one interface in **a, b** Li/Al/LLZTO/Al/Li and **c, d** Li/W/LLZTO/W/Li symmetric cells. The interfaces with interlayers were found to be continuous. The scale bar for **a, c** is 100 $\mu$m and **b, d** is 20 $\mu$m.

## Figure S8

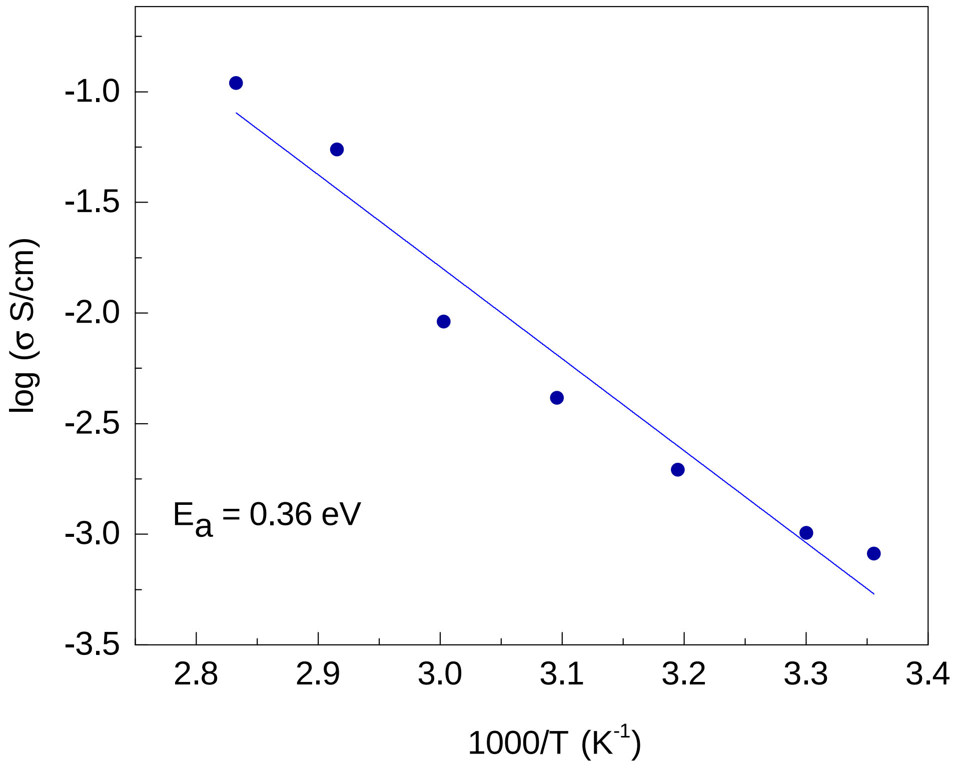


**Fig. S8 | Activation energy for lithium transport in as synthesized LLZTO.** A plot of the logarithm of ionic conductivity versus inverse of temperature for a typical LLZTO pellet. Lithium ionic conductivity measurements were performed at 5 different temperatures of 25, 30, 35, 40, 45 and 50 °C. Activation energy was calculated to be ∼0.36 eV over this temperature range. This is in agreement with previously published values of activation energy for LLZO-based ion conductors (*3*).

**Figure S9**

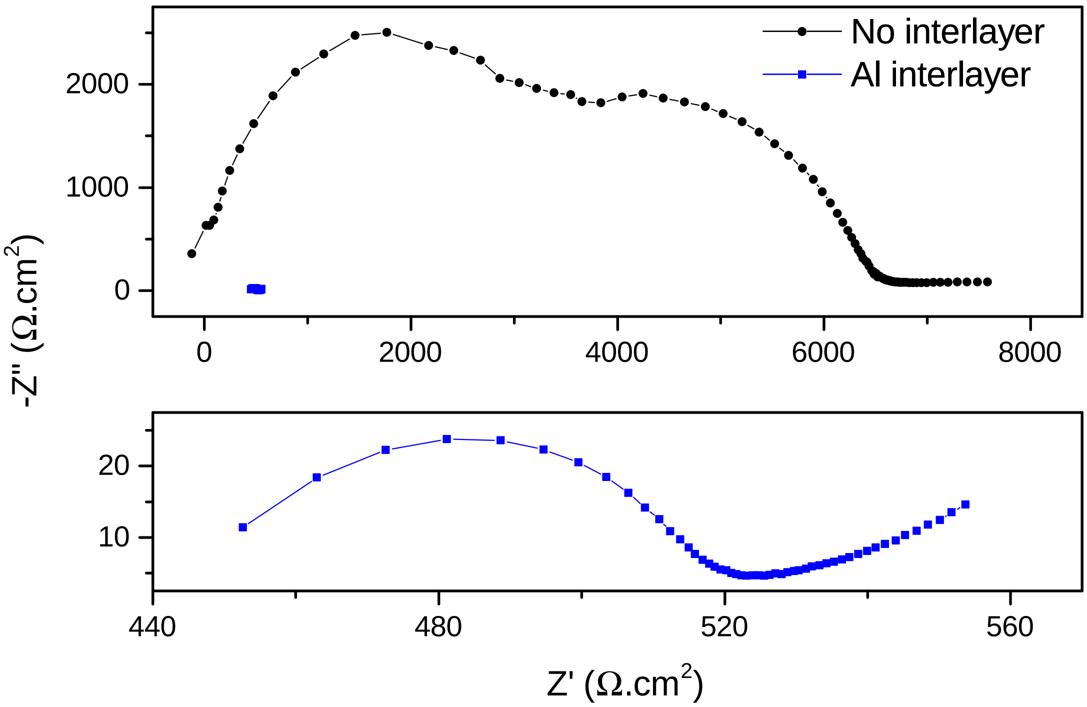


**Fig. S9 | Impedance spectroscopy of symmetric cells with and without aluminum interlayers. a** A typical Nyquist plot comparing the impedance spectra of symmetric Li/LLZTO/Li and Li/Al/LLZTO/Al/Li cells. Clearly, the impedance of the cells with an Al interlayer are lower by more than an order of magnitude in comparison to cells without the interlayer. **b** Impedance data for the Li/Al/LLZTO/Al/Li cell shown in **a**, but plotted over a narrower impedance range for clear resolution of all features of the impedance spectrum. The data was collected on LLZTO pellets that are ∼1 mm in thickness with an AC excitation voltage of 20 mV over a frequency range of 1 Hz to 100 kHz at room temperature.

## Figure S10

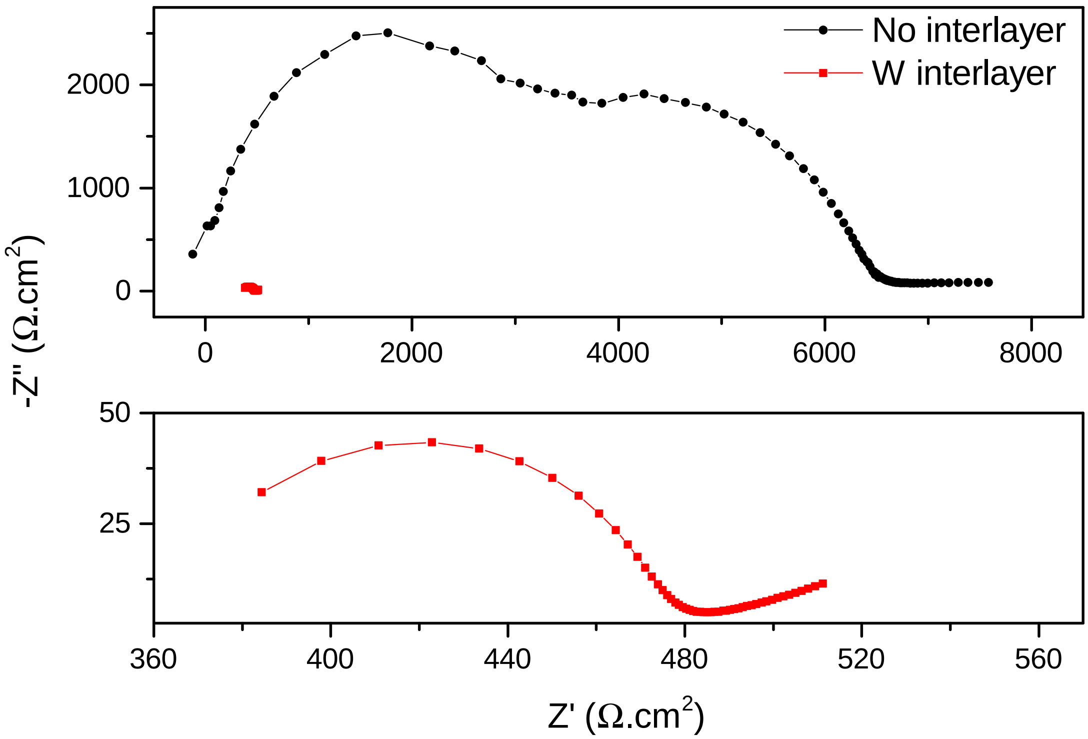


**Fig. S10 | Impedance spectroscopy of symmetric cells with and without tungsten interlayers. a** A typical Nyquist plot comparing the impedance spectra of symmetric Li/LLZTO/Li and Li/W/LLZTO/W/Li cells. Clearly, the impedance of the cells with a W interlayer are lower by more than an order of magnitude in comparison to cells without the interlayer. **b** Impedance data for the Li/W/LLZTO/W/Li cell shown in **a**, but plotted over a narrower impedance range for clear resolution of all features of the impedance spectrum. The data was collected on LLZTO pellets that are ∼1 mm in thickness with an AC excitation voltage of 20 mV over a frequency range of 1 Hz to 100 kHz at room temperature.

## Figure S11

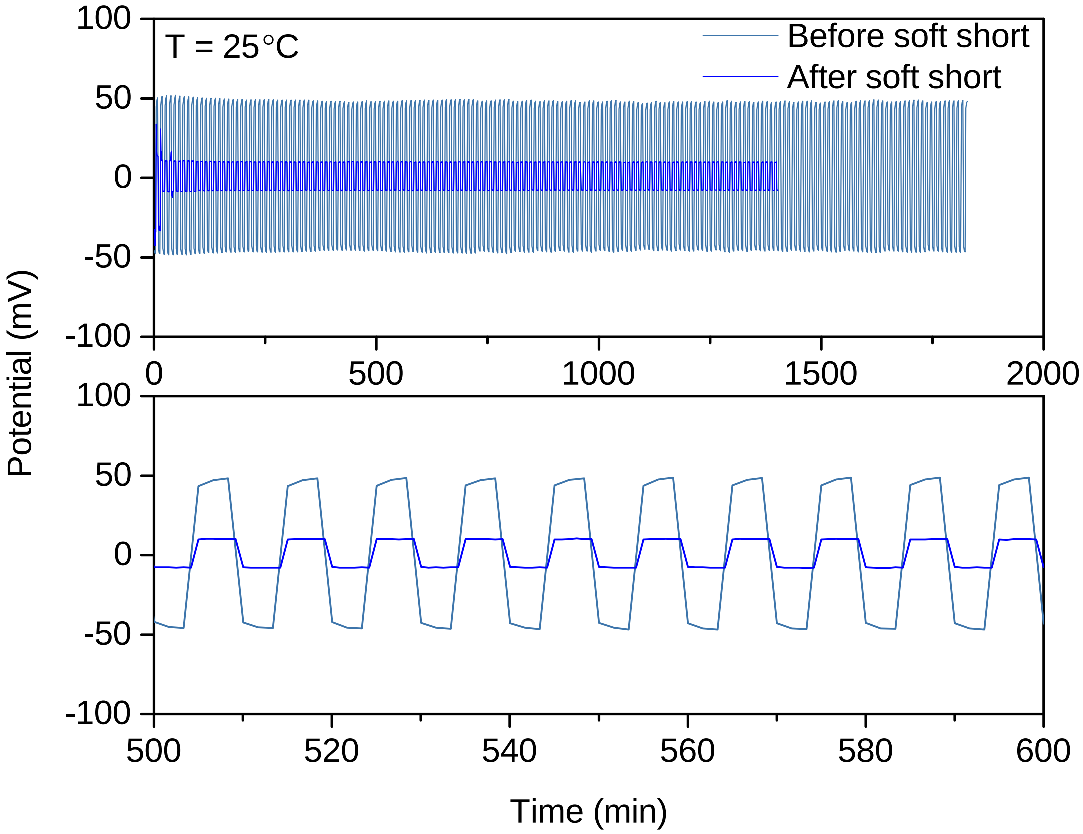


**Fig. S11 | Cells with a soft short show stable cycling. a** A potential versus time plot comparing the potential of a the same cell before and after a short. The potential for plating and stripping seemingly decreases for a cell with a short. **b** The same data as in **a** but plotted over a narrower time scale to clearly show the differences in the potential-times curves before and after a short. There is no voltage polarization observed in the cell with a short, while the same cell before a short shows a small but distinguishable voltage polarization.

## Figure S12

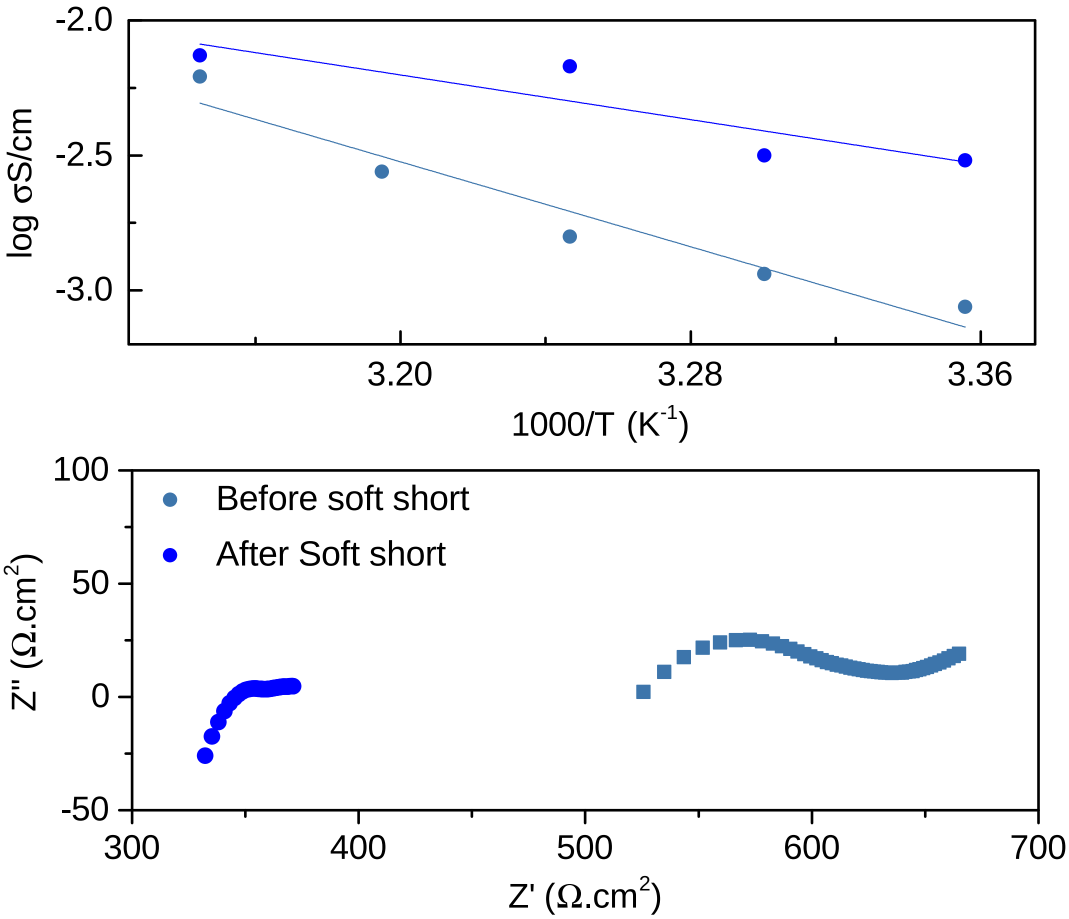


**Fig. S12 | Cells with a soft short show measurable changes in activation energy. a** A comparison of the activation energy for ionic transport in LLZTO pellets in the same cell before and after a short. The calculated activation energy was found to be ∼0.35 eV before the short. This decreases to ∼0.18 eV after the short. Clearly, conduction mechanism seems to have changed (*7*). **b** A typical Nyquist plot comparing the impedance spectra of symmetric Li/W/LLZTO/W/Li cells before and after a short. After a short, a predominant inductive component is observed at high frequencies.

## Figure S13

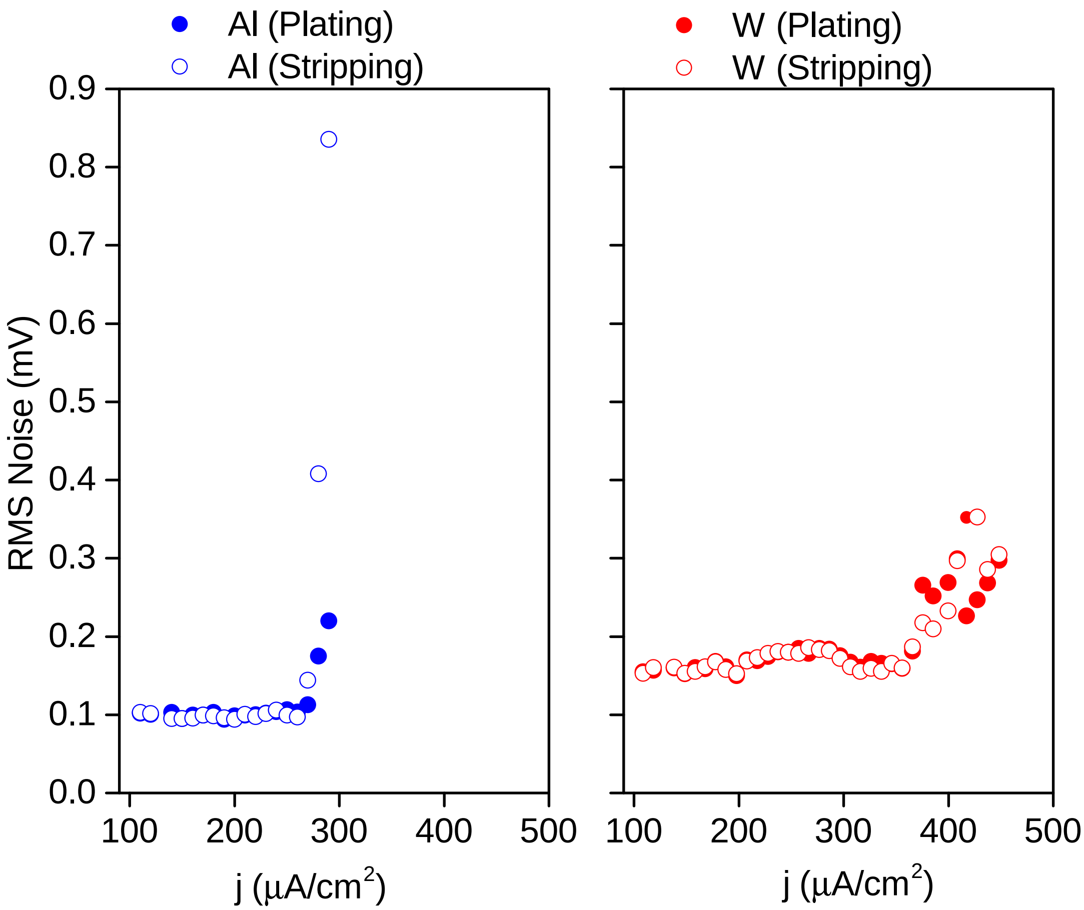


**Fig. S13 | Cells show increased potential noise before a short.** A plot of root-mean-square (RMS) noise in the lithium plating and stripping potentials during a galvanostatic critical current density experiment performed at room temperature for **a** Li/Al/LLZTO/Al/Li and **b** Li/W/LLZTO/W/Li cells. The critical current densities for these Li/Al/LLZTO/Al/Li and Li/W/LLZTO/W/Li cells were found to be 290 $\mu$A/cm$^2$ and 450 $\mu$A/cm$^2$, respectively. Clearly, there is rapid increase in the RMS noise just before the cell shorts.

## Figure S14

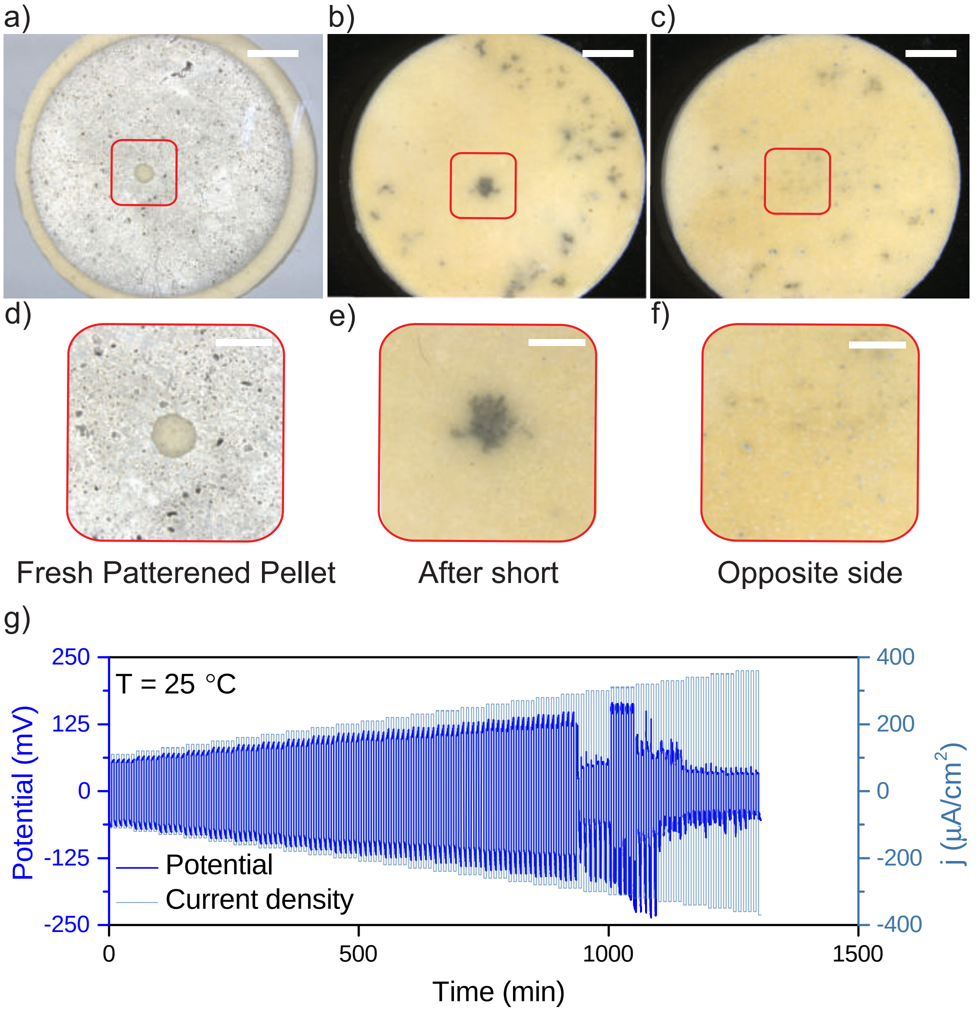


**Fig. S14 | Dendrite growth in cells with a discontinuity in the interlayer.** Optical microscopy image of **a** one side of a pellet with a discontinuity in the aluminum interlayer, **b** the same side and **c** the opposite side of the same pellet as in **a**. Both **b** and **c** are taken on a mechanically polished LLZTO pellet after the cell with the discontinuity is subjected to a galvanostatic critical current density experiment. **d**, **e** and **f** are magnified versions of the optical microscopy images in **a**, **b** and **c**, respectively. The scale bars in **a**, **b** and **c** are equivalent to 2 mm and 1 mm in **d**, **e** and **f**. The black spot in the center of the image in **b** and **e** is taken as indirect evidence for dendrite growth. Such a clear black spot in the vicinity of the discontinuity was not observed on the other side of the pellet. **g.** A plot of potential and current density versus time obtained from the galvanostatic critical current density experiment performed in a symmetric cell employing the LLZTO pellet in **a**.

## Figure S15

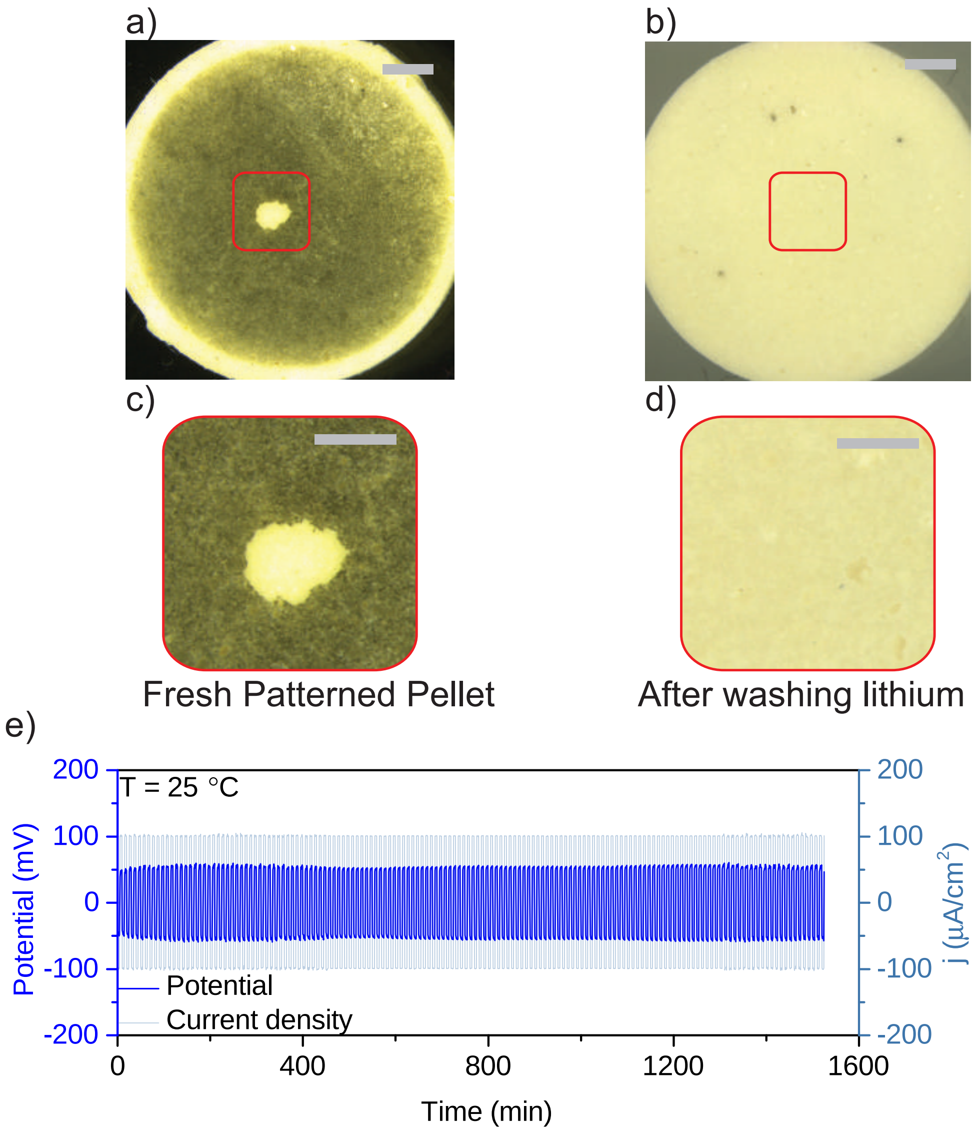


**Fig. S15 | Dendrite growth in cells with a discontinuity in the interlayer.** Optical microscopy image of **a** one side of a pellet with a discontinuity in the aluminum interlayer and **b** the same side of the same pellet as in **a**. **b** is taken on a mechanically polished LLZTO pellet after the cell was cycled at 100 $\mu$A/cm$^2$ but the cycling experiment was stopped before an electrical short. A plot of potential and current density versus time obtained from the galvanostatic cycling experiment performed in a symmetric cell employing the LLZTO pellet in **a**. Clearly, no black spots at the region of the discontinuity can be seen before an electrical short. The scale bars in **a** and **b** are equivalent to 2 mm and 1 mm in **c** and **d**.

## Figure S16

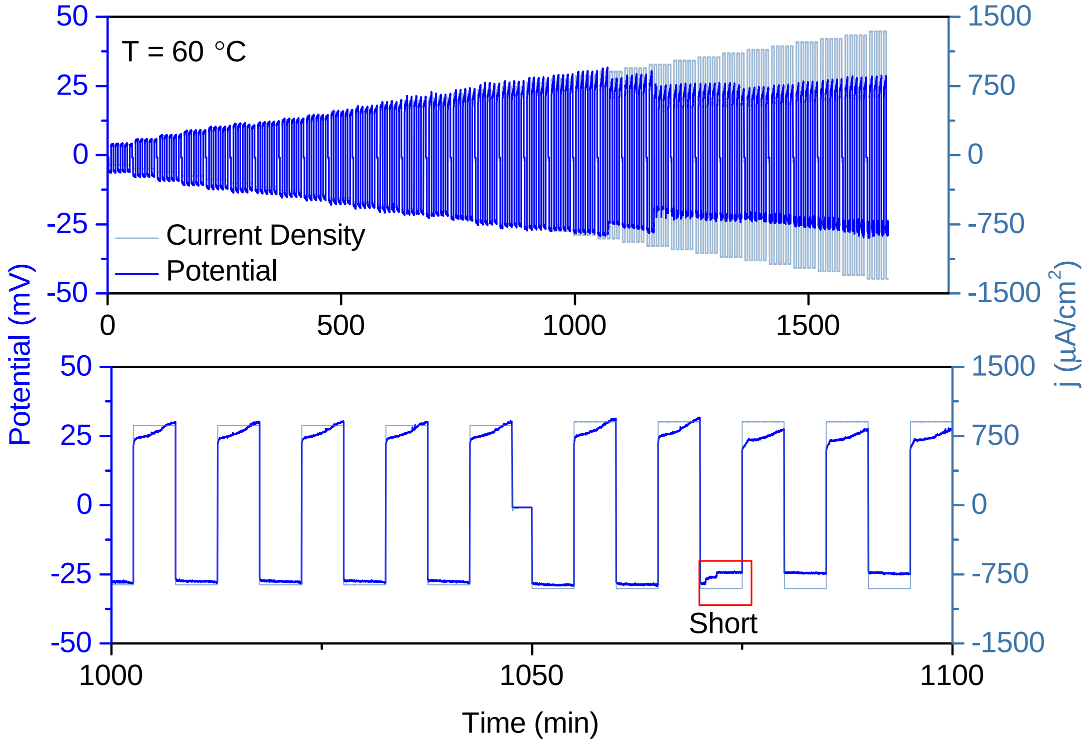


**Fig. S16 | Cells with aluminum Interlayers at 60 °C. a** A typical potential and current density versus time plot obtained from a critical current density experiment performed at a temperature of 60 °C for a symmetric Li/Al/LLZTO/Al/Li cell. **b** The same plot in **a** replotted over a narrower time range to show the potential and current density versus time relationship in the vicinity of a short. This cell shorted at a critical current density of 900 $\mu$A/cm$^2$.

## Figure S17

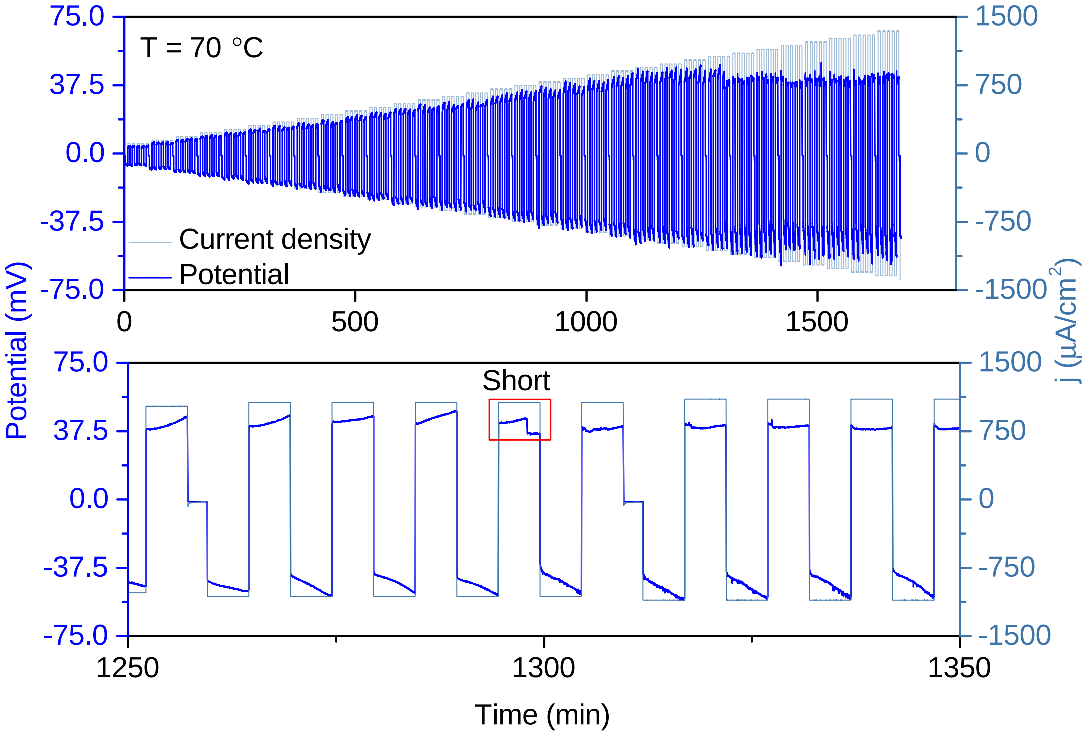


**Fig. 17 | Cells with aluminum Interlayers at 70 °C. a** A typical potential and current density versus time plot obtained from a critical current density experiment performed at a temperature of 70 °C for a symmetric Li/Al/LLZTO/Al/Li cell. **b** The same plot in **a** replotted over a narrower time range to show the potential and current density versus time relationship in the vicinity of a short. This cell shorted at a critical current density of 1030 $\mu$A/cm$^2$.

## Figure S18

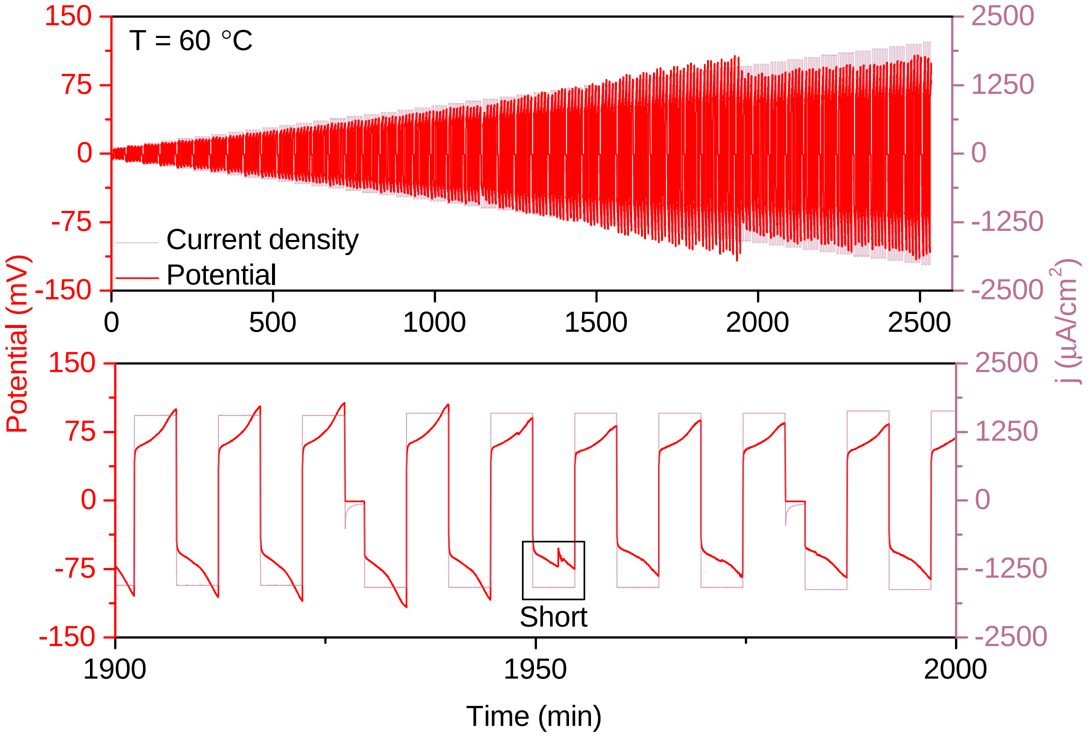


**Fig. S18 | Cells with Tungsten Interlayers at 60 °C. a** A typical potential and current density versus time plot obtained from a critical current density experiment performed at a temperature of 60 °C for a symmetric Li/W/LLZTO/W/Li cell. **b** The same plot in **a** replotted over a narrower time range to show the potential and current density versus time relationship in the vicinity of a short. This cell shorted at a critical current density of 1550 $\mu$A/cm$^2$.

## Figure S19

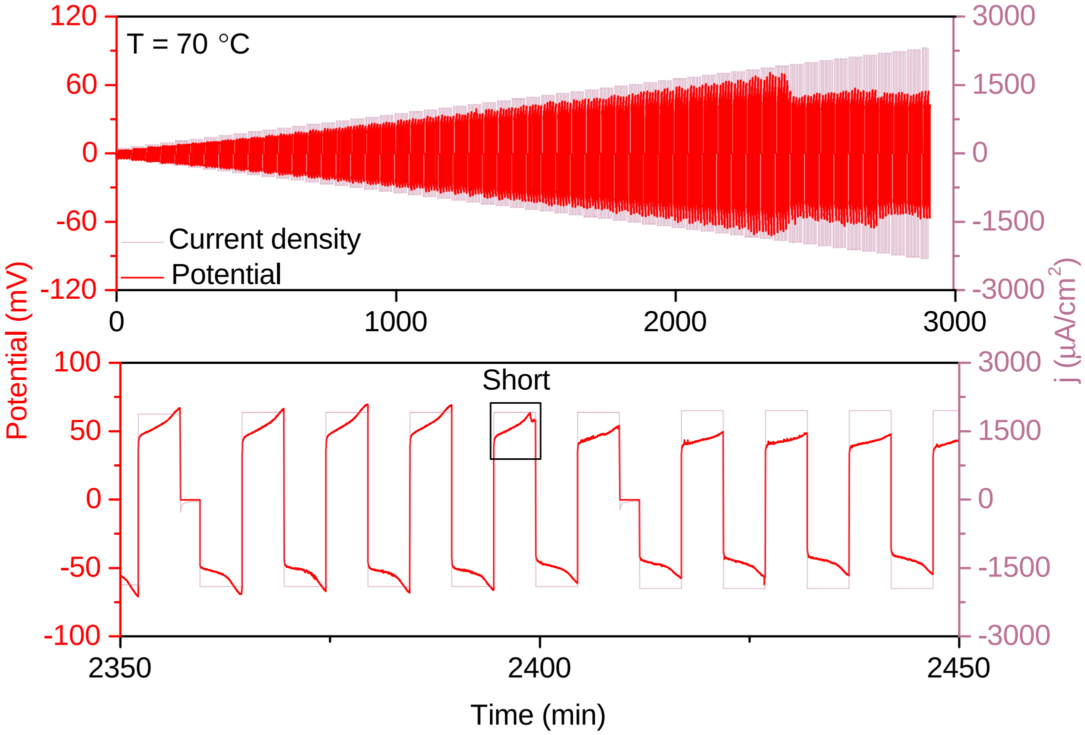


**Fig. S19 | Cells with Tungsten Interlayers at 70 °C. a** A typical potential and current density versus time plot obtained from a critical current density experiment performed at a temperature of 70 °C for a symmetric Li/W/LLZTO/W/Li cell. **b** The same plot in **a** replotted over a narrower time range to show the potential and current density versus time relationship in the vicinity of a short. This cell shorted at a critical current density of 1910 $\mu$A/cm$^2$.

## Figure S20

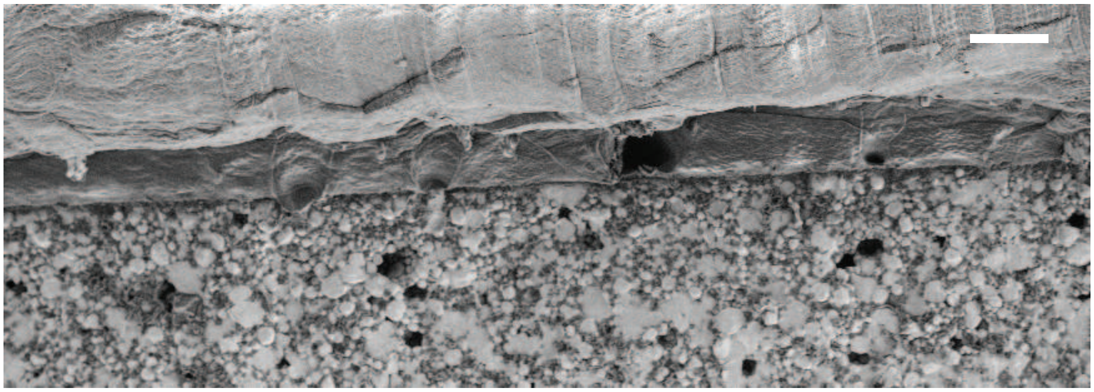

**Fig. S20 | Cross-sectional SEM of Li/W/LLZTO interface.** A cross-sectional SEM at Li/W/LLZTO interface of a shorted cell. Voids at the interface are clearly visible. The scale bar indicates 50 μm.

**Figure S21**

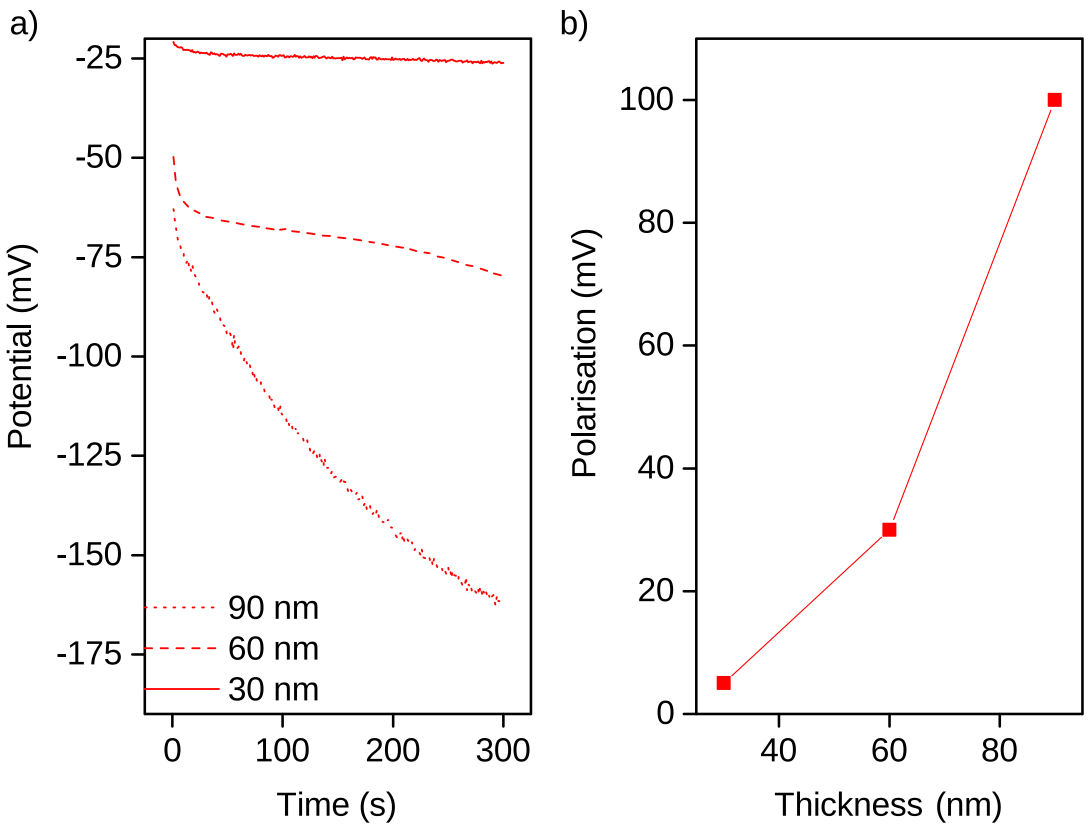


**Fig. S21 | Thickness optimization of tungsten interlayers. a**. A plot of polarization versus time for a lithium plating step for tungsten interlayer thicknesses of 30 nm, 60 nm and 90 nm in Li/W/LLZTO/W/Li symmetric cells. **b**. A plot of total polarization over 300 seconds versus thickness for the cells shown in **a**. Cells with 30 nm of tungsten have the lowest polarization. Therefore all experiments presented in this work used cells employing tungsten interlayers that have a nominal thickness of 30 nm.

## Figure S22

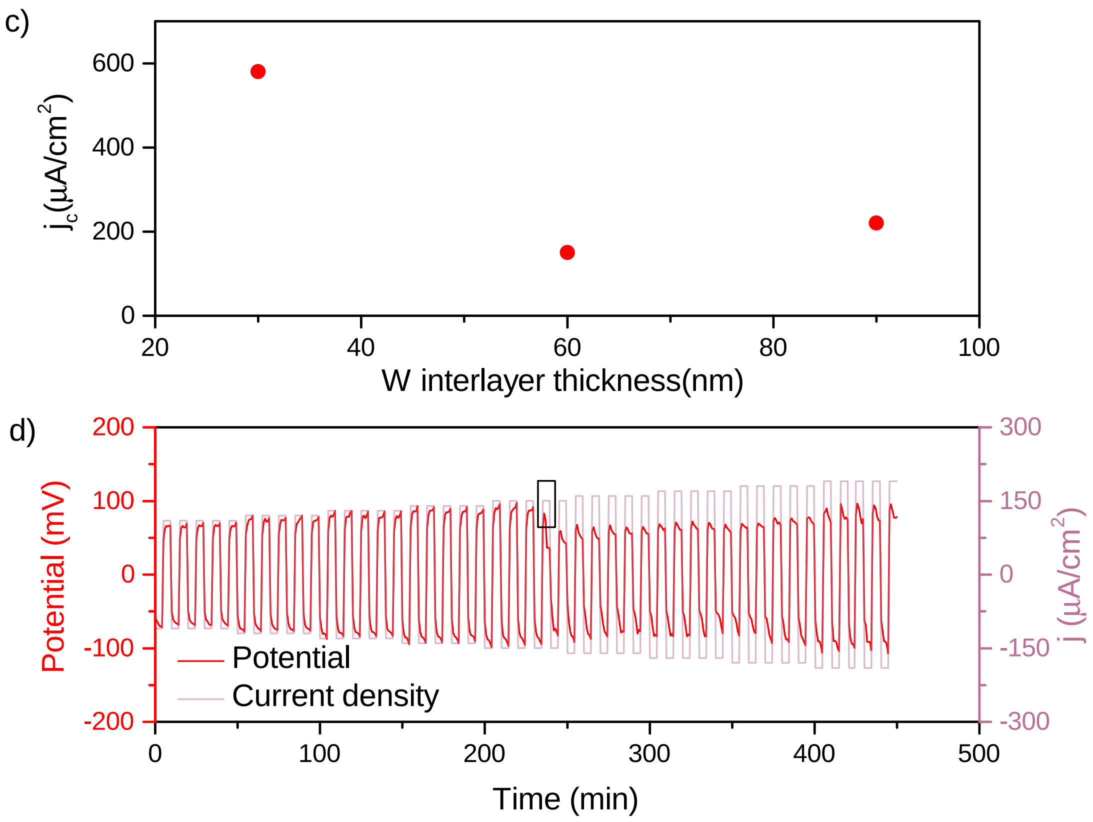


**Fig. S22 | Critical currents at different W interlayer thickness.a** A plot of critical current density for three different W interlayer thickness. We observe higher critical currents at lower thickness. **b** A typical potential and current density versus time plot obtained from a critical current density experiment performed at a temperature of 25 °C for a symmetric Li/W/LLZTO/W/Li cell of thickness 60nm. The critical current density of this cell is 150 $\mu$A/cm$^2$.

# Figure S23

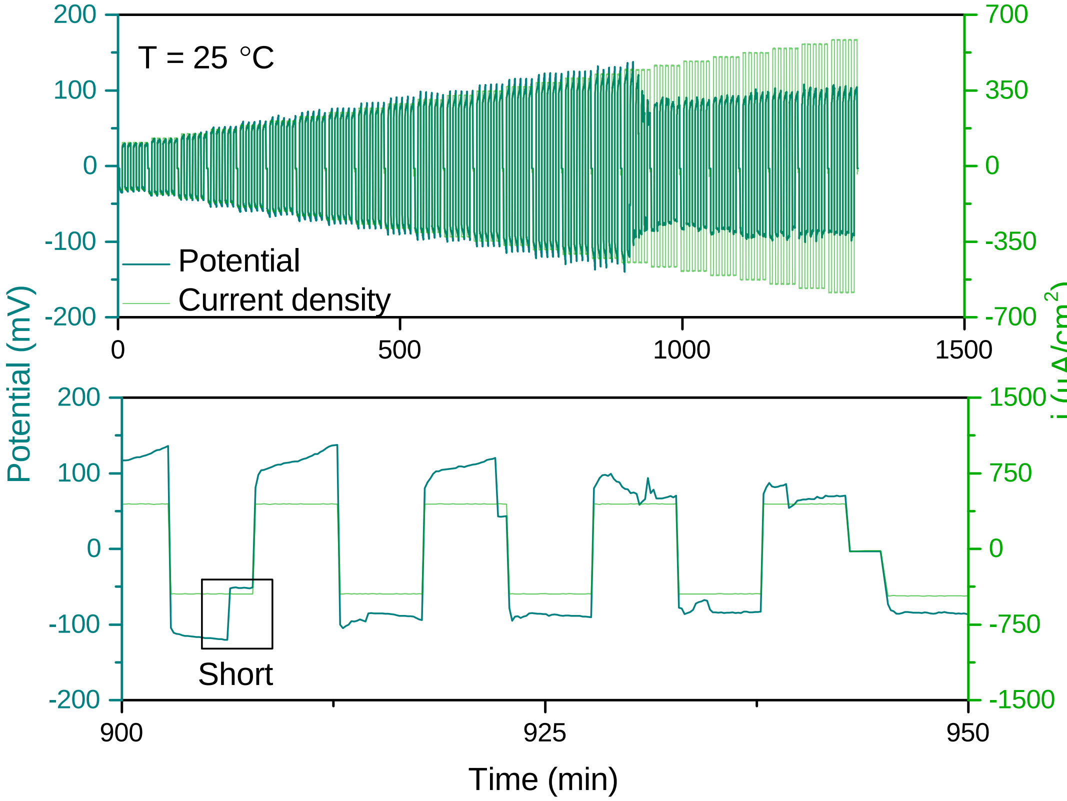


**Fig. S23 | Cells with Molybdenum Interlayers at 25 °C. a** A typical potential and current density versus time plot obtained from a critical current density experiment performed at a temperature of 25 °C for a symmetric Li/Mo/LLZTO/Mo/Li cell. **b** The same plot in **a** replotted over a narrower time range to show the potential and current density versus time relationship in the vicinity of a short. This cell shorted at a critical current density of 450 $\mu$A/cm$^2$. For these experiments, current density is increased in steps of 20 $\mu$A/cm$^2$.

## Figure S24

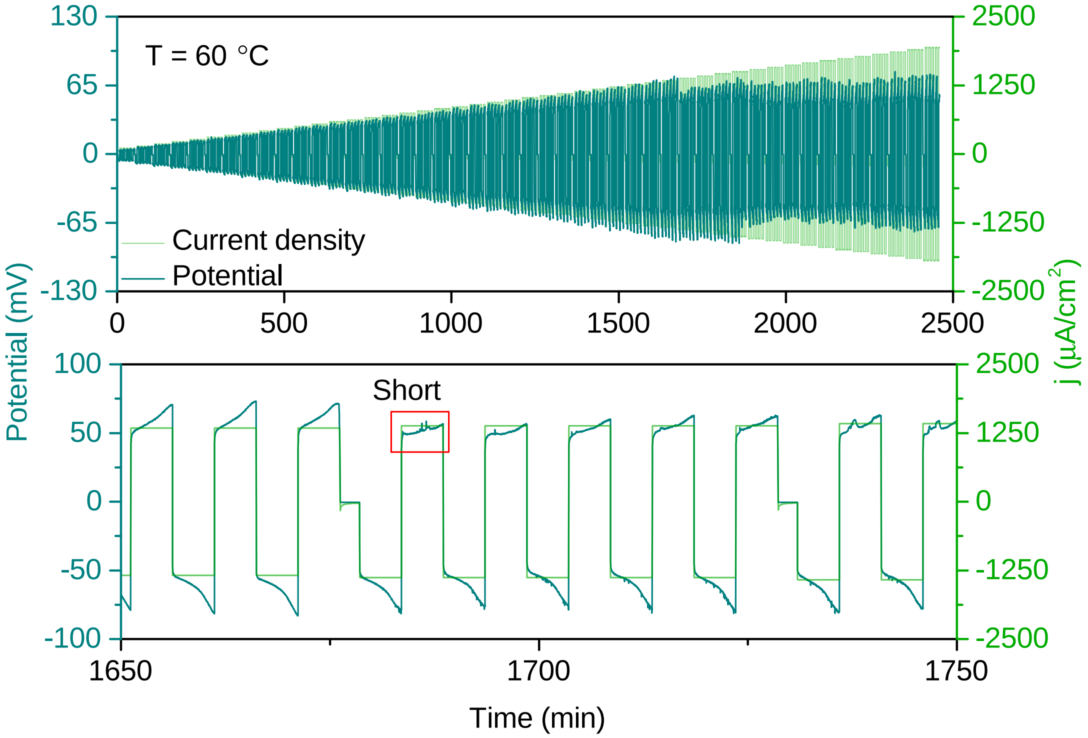


**Fig. S24 | Cells with Molybdenum Interlayers at 60 °C. a** A typical potential and current density versus time plot obtained from a critical current density experiment performed at a temperature of 60 °C for a symmetric Li/Mo/LLZTO/Mo/Li cell. **b** The same plot in **a** replotted over a narrower time range to show the potential and current density versus time relationship in the vicinity of a short. This cell shorted at a critical current density of 1310 $\mu$A/cm$^2$. For these experiments, current density is increased in steps of 20 $\mu$A/cm$^2$.

## Figure S25

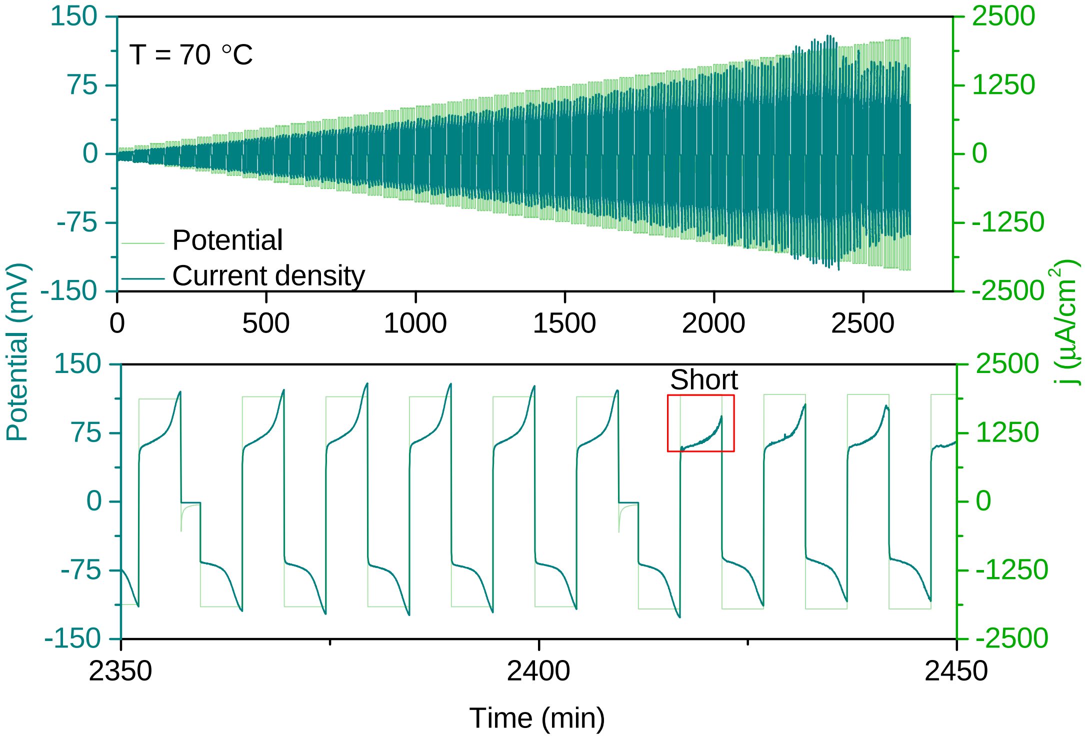


**Fig. S25 | Cells with Molybdenum Interlayers at 70 °C. a** A typical potential and current density versus time plot obtained from a critical current density experiment performed at a temperature of 70 °C for a symmetric Li/Mo/LLZTO/Mo/Li cell. **b** The same plot in **a** replotted over a narrower time range to show the potential and current density versus time relationship in the vicinity of a short. This cell shorted at a critical current density of 1950 $\mu$A/cm$^2$. For these experiments, current density is increased in steps of 20 $\mu$A/cm$^2$.

## Table S2

| Cell No. | Thickness (cm) | Interlayer | Temperature (°C) | Interlayer thickness (nm) | ASR Interfacial (Ohm-cm$^2$) | j ($\mu$A/cm$^2$) |
|---|---|---|---|---|---|---|
| 1 | 0.125 | Al | 25 | 50 | 61.1 | 240 |
| 2 | 0.116 | Al | 25 | 50 | 25.03 | 300 |
| 3 | 0.106 | Al | 25 | 50 | 94.94 | 310 |
| 4 | 0.101 | Al | 25 | 50 | 89.89 | 330 |
| 5 | 0.103 | Al | 25 | 50 | 80.41 | 340 |
| 6 | 0.145 | Al | 25 | 50 | 66.28 | 260 |
| 7 | 0.14 | Al | 25 | 50 | 81.53 | 220 |
| 8 | 0.142 | Al | 25 | 50 | 49.25 | 400 |
| 9 | 0.15 | Al | 25 | 50 | 51.32 | 290 |
| 10 | 0.143 | Al | 25 | 50 | 78.26 | 230 |
| 11 | 0.13 | Al | 25 | 50 | 86.15 | 230 |
| 12 | 0.14 | Al | 25 | 50 | 96.24 | 260 |
| 13 | 0.121 | Al | 25 | 50 | 55.07 | 300 |
| 14 | 0.108 | Al | 25 | 50 | 82.96 | 280 |
| 15 | 0.134 | Al | 25 | 50 | 27.18 | 380 |
| 16 | 0.111 | Al | 25 | 50 | 55.18 | 260 |
| 17 | 0.135 | Al | 25 | 50 | 21.19 | 370 |
| 18 | 0.132 | Al | 25 | 50 | 79.56 | 310 |
| 19 | 0.121 | Al | 25 | 50 | 92.64 | 300 |
| 20 | 0.134 | Al | 25 | 50 | 43.79 | 380 |
| 21 | 0.111 | Al | 25 | 50 | 89.58 | 260 |
| 22 | 0.102 | Al | 25 | 50 | 45.57 | 240 |
| 23 | 0.135 | Al | 25 | 50 | 63.11 | 370 |
| 24 | 0.146 | Al | 25 | 50 | 14.99 | 390 |
| 25 | 0.159 | Al | 25 | 50 | 46.97 | 320 |
| 26 | 0.163 | Al | 25 | 50 | 53.46 | 260 |
| 27 | 0.15039 | Al | 25 | 50 | 65.94 | 290 |
| 28 | 0.118 | W | 25 | 30 | 60.02 | 390 |
| 29 | 0.143 | W | 25 | 30 | 48.01 | 450 |
| 30 | 0.11 | W | 25 | 30 | 40.13 | 530 |
| 31 | 0.108 | W | 25 | 30 | 76.49 | 430 |
| 32 | 0.132 | W | 25 | 30 | 60.15 | 510 |
| 33 | 0.132 | W | 25 | 30 | 45.15 | 580 |
| 34 | 0.118 | W | 25 | 30 | 59.68 | 490 |

| Cell No. | Thickness (cm) | Interlayer | Temperature (°C) | Interlayer thickness (nm) | ASR Interfacial (Ohm-$cm^2$) | j ($\mu$A/$cm^2$) |
|---|---|---|---|---|---|---|
| 35 | 0.107 | W | 25 | 30 | 82.17 | 390 |
| 36 | 0.119 | W | 25 | 30 | 31.77 | 490 |
| 37 | 0.119 | W | 25 | 30 | 51.37 | 500 |
| 38 | 0.151 | W | 25 | 30 | 27.22 | 560 |
| 39 | 0.151 | W | 25 | 30 | 57.22 | 450 |
| 40 | 0.14 | W | 25 | 30 | 29.43 | 480 |
| 41 | 0.097 | W | 25 | 30 | 69.03 | 350 |
| 42 | 0.12 | W | 25 | 30 | 28.32 | 550 |
| 43 | 0.12 | W | 25 | 30 | 33.32 | 430 |
| 44 | 0.137 | W | 25 | 30 | 6.54 | 630 |
| 45 | 0.127 | Al | 60 | 50 | 89.32 | 790 |
| 46 | 0.142 | Al | 60 | 50 | 54.25 | 870 |
| 47 | 0.133 | W | 40 | 30 | 56.55 | 760 |
| 48 | 0.127 | W | 40 | 30 | 96.15 | 630 |
| 49 | 0.12 | Al | 40 | 30 | 46.04 | 650 |
| 50 | 0.137 | W | 60 | 50 | 112.95 | 1270 |
| 51 | 0.144 | W | 60 | 30 | 82.95 | 1440 |
| 52 | 0.143 | W | 60 | 30 | 69.05 | 1350 |
| 53 | 0.105 | Al | 60 | 50 | 132.75 | 600 |
| 54 | 0.112 | W | 60 | 30 | 30.5 | 1350 |
| 55 | 0.109 | Al | 70 | 50 | 16.55 | 1220 |
| 56 | 0.137 | Al | 60 | 50 | 46.62 | 900 |
| 57 | 0.129 | Al | 70 | 50 | 117.75 | 1070 |
| 58 | 0.144 | W | 60 | 30 | 82.95 | 1440 |
| 59 | 0.148 | Al | 40 | 50 | 116.3 | 580 |
| 60 | 0.127 | W | 40 | 30 | 96.15 | 630 |
| 61 | 0.135 | W | 70 | 30 | 86.75 | 1400 |
| 62 | 0.137 | W | 70 | 30 | 70.9 | 1580 |
| 63 | 0.112 | W | 40 | 30 | 60.65 | 670 |
| 64 | 0.137 | Mo | 60 | 30 | 112.95 | 1270 |
| 65 | 0.22 | W | 60 | 30 | 55.9 | 1670 |
| 66 | 0.124 | Al | 40 | 50 | 78.05 | 630 |
| 67 | 0.15 | W | 40 | 30 | 35.12 | 830 |
| 68 | 0.147 | W | 70 | 30 | 36.96 | 1920 |
| 69 | 0.138 | Mo | 60 | 30 | 63.5 | 1310 |
| 70 | 0.149 | Mo | 70 | 30 | 81.6 | 1350 |

| Cell No. | Thickness (cm) | Interlayer | Temperature (°C) | Interlayer thickness (nm) | ASR Interfacial (Ohm-cm$^2$) | j ($\mu$A/cm$^2$) |
|---|---|---|---|---|---|---|
| 71 | 0.15 | Mo | 70 | 30 | 100.6 | 1950 |
| 72 | 0.148 | Al | 70 | 50 | 20.5 | 1250 |
| 73 | 0.108 | Al | 25 | 50 | 91 | 280 |
| 74 | 0.138 | W | 25 | 30 | 31.62 | Long cycling at 400 $\mu$A/cm$^2$ |
| 75 | 0.127 | W | 60 | 30 | 99.34 | Long cycling at 1 mA/cm2 |
| 76 | 0.141 | Mo | 25 | 30 | 46.53 | 450 |
| 77 | 0.148 | Mo | 25 | 30 | 91.76 | 330 |
| 78 | 0.117 | Mo | 25 | 30 | 90.09 | 350 |
| 79 | 0.144 | Mo | 25 | 30 | 57.26 | 470 |
| 80 | 0.145 | Mo | 25 | 30 | 53.74 | 550 |
| 81 | 0.151 | Mo | 25 | 30 | 87.15 | 430 |
| 82 | 0.142 | Mo | 25 | 30 | 63.62 | 510 |

**Table. S2 | Critical current density for all samples used for this study**. A list of all cells measured for this study with thickness of LLZTO, temperature of measurement, interlayer type and thickness, area specific resistance and critical current density.

# References


1. Huang, X. Liu, C. Lu, Y. Xiu, T. Jin, J. E. Badding, M. & Wen, Z. A Li-garnet composite ceramic electrolyte and its solid-state Li-S battery. *Journal of Power Sources* **382**, 190-197 (2017).

2. Thompson, T. *et al.* A tale of two sites: on defining the carrier concentration in garnet-based ionic conductors for advanced Li batteries. *Advanced Energy Materials* **5**, 1500096 (2015).

3. Li, Y. Han, J. T. Wang, C. A. Xie, H. & Goodenough, J. B. Optimizing Li+ conductivity in a

garnet framework. *Journal of Materials Chemistry* **22**, 15357 (2012).

4. Liu, K. Ma, J. T. & Wang, C. A. Excess lithium salt functions more than compensating for lithium loss when synthesizing Li6.5La3Ta0.5Zr1.5O12 in alumina crucible. *Journal of Power Sources* **260**, 109-114 (2014).

5. Huggins, R. A. Simple method to determine electronic and ionic components of the conductivity in mixed conductors a review. *Ionics* **8**, 300 (2002).

6. Han, X. *et al.* Negating interfacial impedance in garnet-based solid-state Li metal batteries. *Nature Materials* **16**, 572-579 (2016).

7. Albertus, P. Babinec, S. Litzelman S. & Newman, A. Status and challenges in enabling the lithium metal electrode for high-energy and low-cost rechargeable batteries. *Nature Energy* **3**, 16-21 (2017).
